# Supplementary material for: Collective inhibition of light scattering from atoms into an optical cavity at a magic frequency
Source: arXiv:2601.08978 source file (2026-01-13)
Supplement: Supplementary file 1 [file Magic_wavelengths___supplement.pdf]

# Collective inhibition of light scattering from atoms into an optical cavity at a magic frequency: supplemental document

## 1. TRANSITION RATES OF CAVITY PHOTON SCATTERING FROM A SINGLE ATOM

Light scattering from coherently laser-driven atoms into two, near resonant degenerate cavity modes $a_y$ and $a_z$, with orthogonal linear polarizations $\vec{y}$ and $\vec{z}$, is described by the single-atom Hamiltonian, written with respect to the quantization axis $\vec{z}$,

$$\begin{aligned} H_0 &= -\Delta_c \left(a_z^\dagger a_z + a_y^\dagger a_y\right) - \sum_{m',F'} \Delta_{F'} \left|F',m'\right\rangle\!\left\langle F',m'\right| \\ H_{\mathrm{cav}} &= ig\cos(k_c x) \sum_{m,F'} \Big[ a_z^\dagger c_{F';m,m} \left|F,m\right\rangle\!\left\langle F',m\right| \\ &\quad + \frac{i}{\sqrt{2}} a_y^\dagger \Big( c_{F';m,m-1} \left|F,m\right\rangle\!\left\langle F',m-1\right| + c_{F';m,m+1} \left|F,m\right\rangle\!\left\langle F',m+1\right| \Big)\Big] + \mathrm{H.c.} \\ H_{\mathrm{drive}} &= i\eta_+ \sum_{m,F'} e^{-ikz} c_{F';m,m+1} \left|F,m\right\rangle\!\left\langle F',m+1\right| + i\eta_- \sum_{m,F'} e^{ikz} c_{F';m,m-1} \left|F,m\right\rangle\!\left\langle F',m-1\right| + \mathrm{H.c.}\,. \end{aligned} \tag{S1}$$

The atomic center-of-mass degrees of freedom are described by the coordinates $x$ and $z$, while the internal atomic degrees of freedom are given by the hyperfine manifolds $F = 2$ in the ground state and $F' = 1, 2, 3$ in the excited state, along with the magnetic quantum numbers $m$. Dipole-allowed transitions $|F,m\rangle \leftrightarrow |F',m'\rangle$, characterized by the Clebsch–Gordan coefficients $c_{F';m,m'}$, couple to the cavity modes via $H_{\mathrm{cav}}$ with coupling strength $g$, and to the coherent drive via $H_{\mathrm{drive}}$ with drive amplitudes $\eta_\pm$ corresponding to the $\sigma^\pm$-polarized beams. The detunings are defined as $\Delta_c = \omega - \omega_c$ for the cavity and $\Delta_{F'} = \omega - \omega_{F'}$ for the atomic transitions. The coherent drive and cavity fields have frequencies $\omega$ and $\omega_c$, and wave numbers $k$ and $k_c$, respectively, while $\omega_F$ denotes the atomic transition frequency associated with the hyperfine level $F$. In the absence of an external magnetic field, the Zeeman sublevels within each hyperfine manifold are taken to be degenerate.

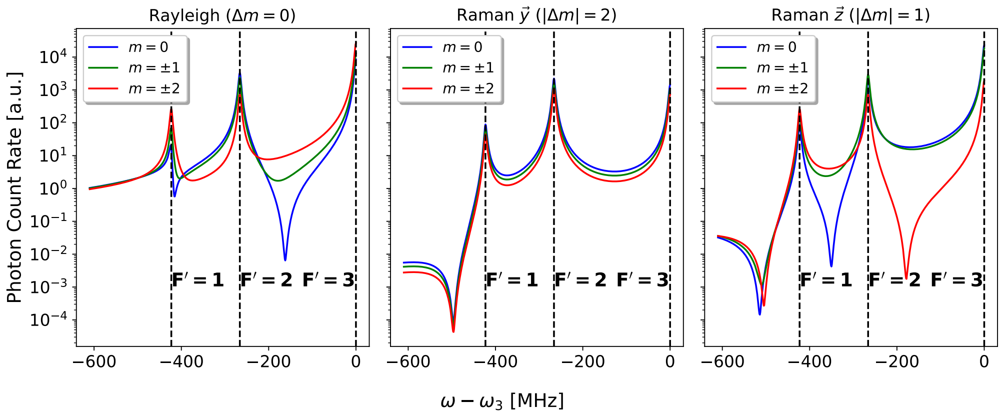


**Fig. S1.** Zeeman-sublevel-resolved photon rates, computed from the single atom two-photon transition amplitudes (S3-S5) for the Rayleigh and Raman channels in the vicinity of the three excited hyperfine levels $F' = 1, 2, 3$.

Within the framework of second-order perturbation theory, under the condition $\Delta_{F'} \gg g, \eta_\pm$, the two-photon scattering amplitudes

$$S^{\Delta m}_{m;y(z)} = \sum_{F',m'} \frac{\left\langle F, m+\Delta m; 1_{y(z)} \middle| H_{\text{cav}} \middle| F', m'; 0 \right\rangle \langle F', m'; 0 | H_{\text{drive}} | F, m; 0 \rangle}{\Delta_{F'} + i\gamma_{F'}}, \tag{S2}$$

describe the allowed scattering channels with $\Delta m \in 0, \pm 1, \pm 2$, connecting an initial atomic Zeeman sublevel $m$ with empty cavity modes, $|F, m; 0\rangle$, to the final state $\left|F, m+\Delta m; 1_{y(z)}\right\rangle$, in which the magnetic quantum number changes by $\Delta m$ and one excitation appears in either the $\vec{y}$ or $\vec{z}$-polarized cavity mode through the interactions $H_{\text{drive}}$ and $H_{\text{cav}}$. Here, $\gamma_{F'}$ denotes the spontaneous decay rate of the excited hyperfine level. Explicitly, the scattering amplitudes read

$$S^0_{m;y}(\vec{r}) = \frac{i}{\sqrt{2}} g \cos(k_c x) \left( \eta_+ e^{ikz} \sum_{F'} \frac{c^2_{F';m,m+1}}{\Delta_{F'} + i\gamma_{F'}} + \eta_- e^{-ikz} \sum_{F'} \frac{c^2_{F';m,m-1}}{\Delta_{F'} + i\gamma_{F'}} \right), \tag{S3}$$

$$S^{\pm 1}_{m;z}(\vec{r}) = g \cos(k_c x) \eta_\pm e^{\pm ikz} \sum_{F'} \frac{c_{F';m,m\pm 1} c_{F';m\pm 1,m\pm 1}}{\Delta_{F'} + i\gamma_{F'}}, \tag{S4}$$

$$S^{\pm 2}_{m;y}(\vec{r}) = \frac{i}{\sqrt{2}} g \cos(k_c x) \eta_\pm e^{\pm ikz} \sum_{F'} \frac{c_{F';m,m\pm 1} c_{F';m\pm 2,m\pm 1}}{\Delta_{F'} + i\gamma_{F'}}. \tag{S5}$$

The intensity of the $\vec{y}$-polarized cavity field arising from Rayleigh scattering from a given magnetic sublevel $m$, where the $\sigma^+$ and $\sigma^-$ transition pathways contribute coherently, is given by $W^0_{m;y} = \left|S^0_{m;y}\right|^2$. Raman processes contribute to both $\vec{y}$ and $\vec{z}$ polarized cavity fields, with rates $W^{|\Delta m|=2}_{m;y} = \sum_{\Delta m = \pm 2} \left|S^{\Delta m}_{m;y}\right|^2$ and $W^{|\Delta m|=1}_{m;z} = \sum_{\Delta m = \pm 1} \left|S^{\Delta m}_{m;z}\right|^2$.

The resulting $m$-resolved scattering rates for the three scattering processes are shown in fig. S1. For simplicity, the spatial dependence has been neglected by evaluating the amplitudes at $\vec{r} = 0$. Strong suppression of scattering arises from destructive interference among the three excitation pathways via the excited hyperfine states at nontrivial detunings that are entirely determined by the Clebsch–Gordan coefficients. These magic detunings occur in both Rayleigh and Raman channels; however, a uniform suppression across all magnetic sublevels is observed only for the Raman processes, at a detuning of $-506$ MHz. For an ensemble of $N$ atoms, the total scattered intensity is obtained by summing the scattering rates of the individual atoms at positions $\vec{r}_a$. Assuming a uniform spatial distribution and a completely mixed population over the ground-state magnetic sublevels, the ensemble-averaged scattering rates, obtained by substituting the appropriate Clebsch–Gordan coefficients, read

$$\begin{aligned}
W_{\text{Rayleigh}} &= \sum_{a=1}^{N} \frac{1}{5} \sum_m W^0_{m;y}(\vec{r}_a) \\
&= \frac{g^2(\eta_+^2 + \eta_-^2) N_{\text{eff}}}{10} \left( \frac{23/1800}{\Delta_1^2 + \gamma_1^2} + \frac{13/72}{\Delta_2^2 + \gamma_2^2} + \frac{371/225}{\Delta_3^2 + \gamma_3^2} + \frac{1/15}{\Delta_{12}^2} + \frac{7/150}{\Delta_{13}^2} + \frac{49/90}{\Delta_{23}^2} \right), \\
W_{\text{Raman,y}} &= \sum_{a=1}^{N} \frac{1}{5} \sum_m W^{|\Delta m|=2}_{m;y}(\vec{r}_a) \\
&= \frac{g^2(\eta_+^2 + \eta_-^2) N_{\text{eff}}}{10} \left( \frac{7/1200}{\Delta_1^2 + \gamma^2} + \frac{7/48}{\Delta_2^2 + \gamma^2} + \frac{7/75}{\Delta_3^2 + \gamma^2} - \frac{7/120}{\Delta_{12}^2} - \frac{7/30}{\Delta_{23}^2} + \frac{7/150}{\Delta_{13}^2} \right), \\
W_{\text{Raman,z}} &= \sum_{a=1}^{N} \frac{1}{5} \sum_m W^{|\Delta m|=1}_{m;z}(\vec{r}_a) \\
&= \frac{g^2(\eta_+^2 + \eta_-^2) N_{\text{eff}}}{5} \left( \frac{11/1200}{\Delta_1^2 + \gamma^2} + \frac{13/144}{\Delta_2^2 + \gamma^2} + \frac{133/225}{\Delta_3^2 + \gamma^2} - \frac{1/120}{\Delta_{12}^2} - \frac{14/45}{\Delta_{23}^2} + \frac{7/75}{\Delta_{13}^2} \right).
\end{aligned} \tag{S6}$$

Here, the effective detunings appearing in the cross terms are defined as

$$\Delta^{-2}_{F'F''} = (\Delta_{F'} \Delta_{F''} + \gamma_{F'} \gamma_{F''}) \left[ (\Delta_{F'} \Delta_{F''} + \gamma_{F'} \gamma_{F''})^2 + (\Delta_{F'} \gamma_{F'} - \Delta_{F''} \gamma_{F''})^2 \right]^{-1},$$

and the effective atom number is given by $N_{\text{eff}} = \sum_a \cos^2(k_c x_a)$. The total $\vec{y}$- and $\vec{z}$-polarized signals, $W_y = W_{\text{Rayleigh}} + W_{\text{Raman,y}}$ and $W_z = W_{\text{Raman,z}}$, exhibit a detuning-dependent polarization rotation, in good agreement with the measured ratios shown in fig. S2. Notably, this ratio contains no free fitting parameters, in contrast to the individual scattering rates presented in fig. 2 of the Main Text. The photon emission rates into the $\vec{y}$- and $\vec{z}$-polarized cavity modes contribute comparably to the total scattering rate. However, for detunings below –450 MHz, the $m$-independent suppression of Raman scattering causes the $\vec{y}$-polarized rate to exceed the $\vec{z}$-polarized rate by a few orders of magnitude.

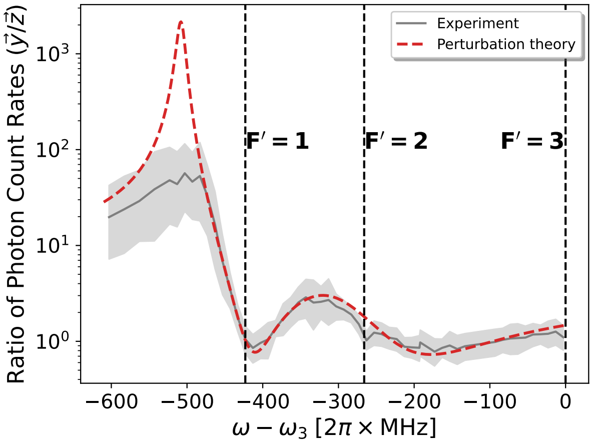


**Fig. S2.** Ratio of the photon count rates in the two cavity polarizations as a function of the drive detuning. The measurement data (solid lines with shaded area representing the width of the distribution at half maximum) are compared with the single-atom scattering rate model (dashed line).

## 2. COLLECTIVE ATOM-CAVITY COUPLING

In this section, we will describe the interaction of an ensemble of $N$ atoms with the two orthogonal cavity modes in the strong collective coupling regime. Compared to the single-atom approach leading to the previous calculation of scattering rates, here the simultaneous effect of the atoms on the cavity field is taken into account.

For all the atoms in the ensemble, indexed by $a = 1$, let us define a set of atomic polarization operators, both along the $\vec{y}$ and $\vec{z}$ directions,

$$d^y_{m_a,F'} = \frac{i}{\sqrt{2}}\left(c_{F';m_a,m_a-1}\left|F,m_a\right\rangle\!\left\langle F',m_a-1\right| + c_{F';m_a,m_a+1}\left|F,m_a\right\rangle\!\left\langle F',m_a+1\right|\right), \tag{S7}$$

$$d^z_{m_a,F'} = c_{F';m_a,m_a}\left|F,m_a\right\rangle\!\left\langle F',m_a\right| , \tag{S8}$$

which are associated with the transitions to the excited manifold $F' = 1,2,3$. The atom labeled $a$ is assumed to be initially in the Zeeman state $m_a$ of the ground state manifold $F$. Rather than considering a mixed ground state for each atom, it is equivalent to consider each atom in a given random sublevel $m_a$ such that the large ensemble realizes the actual population distribution.

The full Hamiltonian leads to the linearized Heisenberg equations of motion for the individual atomic polarizations and the cavity field mode amplitudes

$$\begin{aligned}\frac{d}{dt}d^y_{m_a,F'}(\vec{r}_a) = (i\Delta_{F'} - \gamma_{F'})d^y_{m_a,F'}(\vec{r}_a) - g\cos(k_c x_a)a_y\frac{1}{2}\left(c^2_{F';m_a,m_a+1} + c^2_{F';m_a,m_a-1}\right)\\ - i\eta\cos(kz_a)\frac{1}{2}\left(c^2_{F';m_a,m_a+1} + c^2_{F';m_a,m_a-1}\right),\end{aligned} \tag{S9a}$$

$$\frac{d}{dt}a_y = (i\Delta_c - \kappa)a_y + g\sum_{a=1}^{N}\left(\cos(k_c x_a)\sum_{F'} d^y_{m_a,F'}(\vec{r}_a)\right), \tag{S9b}$$

in the $y$ direction, where the spontaneous emission and the cavity decay terms are included. The corresponding Langevin noise terms can be omitted since we will consider later only the

mean field. The atomic drive term in the second line of the first equation was written for the case of symmetric illumination, i.e. $\eta \equiv \sqrt{2}\eta_+ = \sqrt{2}\eta_-$, corresponding to our experimental configuration. Decoupled from this polarization, there are similar equations in the $z$ direction,

$$\frac{d}{dt} d^z_{m_a,F'}(\vec{r}_a) = (i\Delta_{F'} - \gamma_{F'}) d^z_{m_a,F'}(\vec{r}_a) - g\cos(k_c x_a) a_z c^2_{F';m_a,m_a}\,, \tag{S9c}$$

$$\frac{d}{dt} a_z = (i\Delta_c - \kappa) a_z + g \sum_{a=1}^{N} \left( \cos(k_c x_a) \sum_{F'} d^z_{m_a,F'}(\vec{r}_a) \right). \tag{S9d}$$

These equations form a closed set only because of the linearization. Besides neglecting the population in the excited atomic states $F'$, as is usual in the low-saturation limit of two-level atoms, here the coherence between different Zeeman states of the ground state multiplet (and, obviously, for the excited one) are also neglected.

Each of the two sets of equations contains $3N+1$ coupled variables. The factor 3 comes from the number of relevant excited hyperfine states, $F' = 1, 2, 3$. The coupled linear equations can be diagonalized in terms of normal modes. Among them, there are two normal modes, *the polaritons*, which mix the cavity and the atomic degrees of freedom. The polaritons underlie our experimental observations on the cavity output photon rates. Rather than solving the full algebraic problem, we will consider the polaritons in the limit of large atomic detuning, being of interest for the observed dip at $\Delta_{3'} = -2\pi \times 185$ MHz, $\Delta_{2'} = 2\pi \times 80$ MHz and $\Delta_{1'} = 2\pi \times 230$ MHz. In this limit the polaritons are manifest in simple modified equations describing the cavity modes dressed by the corresponding atomic polarizations.

The fast dynamics of the atomic polarizations can be adiabatically eliminated to get the steady states

$$d^y_{m_a,F'}(\vec{r}_a) = \big(a_y g \cos(k_c x_a) + i\eta \cos(k z_a)\big) \frac{c^2_{F';m_a,m_a+1} + c^2_{F';m_a,m_a-1}}{2(i\Delta_{F'} - \gamma_{F'})}\,, \tag{S10a}$$

$$d^z_{m_a,F'}(\vec{r}_a) = a_z g \cos(k_c x_a) \frac{c^2_{F';m_a,m_a}}{i\Delta_{F'} - \gamma_{F'}}\,. \tag{S10b}$$

In accordance with eq. (S9), the sum of these polarizations to the different $F'$ excited states, weighted by the atomic position and Zeeman ground state distributions yields the collective atomic source terms for the cavity modes $\vec{y}$ and $\vec{z}$, respectively,

$$\begin{aligned}\sum_{a=1}^{N} \cos(k_c x_a) \sum_{F'} d^y_{m_a,F'}(\vec{r}_a) &= \sum_{a=1}^{N} \big(a_y g \cos(k_c x_a) + i\eta \cos(k z_a)\big) \cos(k_c x_a) \\ &\qquad \times \sum_{F'} \frac{c^2_{F';m_a,m_a+1} + c^2_{F';m_a,m_a-1}}{2(i\Delta_{F'} - \gamma_{F'})} \\ &= a_y N_{\mathrm{eff}} g\, \mathcal{P}(\Delta) + i\eta\, \mathcal{P}(\Delta) \sum_{a=1}^{N} \cos(k z_a) \cos(k_c x_a)\,, \end{aligned} \tag{S11a}$$

$$\begin{aligned}\sum_{a=1}^{N} \cos(k_c x_a) \sum_{F'} d^z_{m_a,F'}(\vec{r}_a) &= a_z g \sum_{a=1}^{N} \cos^2(k_c x_a) \sum_{F'} \frac{c^2_{F';m_a,m_a}}{i\Delta_{F'} - \gamma_{F'}} \\ &= a_z N_{\mathrm{eff}} g\, \mathcal{P}(\Delta)\,, \end{aligned} \tag{S11b}$$

where the effective atom number $N_{\mathrm{eff}} = \sum_{a=1}^{N} \cos^2(k_c x_a) \approx N/2$. Atomic interference represented by the summation over the excited hyperfine states $F'$ is embedded in the collective polarization $\mathcal{P}(\Delta = \omega - \omega_3)$. Simultaneously, the summation for the atoms $a = 1 \dots N$ involves the averaging over the ground-state Zeeman sublevels. This leads to an averaging in the collective polarization function,

$$\mathcal{P}(\Delta) = \sum_{F'} \frac{\langle c^2_{F'} \rangle}{i\Delta_{F'} - \gamma_{F'}}\,. \tag{S12}$$

When the ground state distribution is close to uniform, the polarization functions in the $\vec{y}$ and $\vec{z}$ directions are the same, that is,

$$\left\langle c^2_{F'} \right\rangle \equiv \tfrac{1}{5} \sum_m c^2_{F';m,m} = \tfrac{1}{5} \sum_m c^2_{F';m,m\pm1}\,. \tag{S13}$$

We can safely assume that the atomic population was evenly distributed among the Zeeman sublevels, which holds for a thermal ensemble in the given isotropic environment. Optical pumping processes due to the laser drives can only slightly alter this distribution in steady-state.

Inserting the adiabatic solutions for the atomic polarizability into the cavity field mode equations, the polariton equations of motion are obtained as

$$\frac{d}{dt}a_y = \left(i\Delta_c - \kappa + N_{\text{eff}}g^2\,\mathcal{P}(\Delta)\right)a_y + i\eta g\,\mathcal{P}(\Delta)\sum_{a=1}^{N}\cos(kz_a)\cos(k_c x_a)\,, \tag{S14a}$$

$$\frac{d}{dt}a_z = \left(i\Delta_c - \kappa + N_{\text{eff}}g^2\,\mathcal{P}(\Delta)\right)a_z\,. \tag{S14b}$$

The complex frequency term shows that the polaritons have a non-trivial spectrum which depends on the collective atomic polarizability function $\mathcal{P}(\Delta)$. Nevertheless, this spectrum is the same for the $\vec{y}$ and $\vec{z}$ polarized polaritons.

Only the $\vec{y}$ polariton is driven coherently, expressed by the drive term above. This drive involves spatial interference $\sum_{a=1}^{N}\cos(kz_a)\cos(k_c x_a)$ for the components originating from the different atoms. For uniform spatial distribution of the atoms the mean field scattered from the drive laser vanishes. This effect is also known as the normal phase of the spatial self-organization of atoms in a cavity [1]. The uniform distribution becomes unstable above a certain critical drive power ($\propto \eta^2$). However, even below the threshold, there are density fluctuations around the uniform distribution, which results in an incoherent scattering into the cavity with an intensity proportional to the number of atoms (as opposed to the scaling $\propto N^2$ characteristic of superradiant scattering). So the $\vec{y}$ polarized polariton is excited as it has been experimentally demonstrated in the case of the vacuum Rabi splitting [2].

Accordingly, the steady-state intracavity photon number is

$$\left|a_y\right|^2 = \eta^2 g^2 \mathcal{S}\frac{|\mathcal{P}(\Delta)|^2}{|i\Delta_c - \kappa + g^2 N_{\text{eff}}\mathcal{P}(\Delta)|^2}\,, \tag{S15}$$

where $\mathcal{S} = \left|\sum_{a=1}^{N}\cos(k_c x_a)\cos(kz_a)\right|^2 \approx N/4$ for a quasi-uniform spatial distribution of atoms corresponding to the configuration of our experimental scheme. This result is used as Eq. (3) of the paper.

The numerator in Eq. S15 shows explicitly that scattering into the $\vec{y}$-polarized cavity mode is collectively suppressed by destructive interference encoded in $\mathcal{P}(\Delta)$. The main point is that the suppression occurs at the level of the polariton, i.e., the specific drive frequency satisfying $\mathcal{P}(\Delta) = 0$ does not imply a destructive interference at the single atom level for arbitrary $m_a$ magnetic sublevel.

At the same time, the atomic dispersive shift $g^2 N_{\text{eff}}\mathcal{P}(\Delta)$ of the cavity response vanishes, reflecting the decoupling of the polariton from the cavity. Near the magic detuning $\Delta^*$, defined by $\mathcal{P}(\Delta^*) = 0$, and neglecting absorptive contributions, the polarization function can be linearized as

$$\mathcal{P}(\Delta = \Delta^* + \delta) \simeq -ip_1\delta\,, \tag{S16}$$

with the linear coefficient $p_1 = \left(\Delta_1^*\Delta_2^*\Delta_3^*\right)^{-1}\sum_{F'}\left\langle c_{F'}^2\right\rangle\sum_{j\neq F'}\Delta_j^*$, where $\Delta_j^*$ denote the magic detunings relative to the three excited hyperfine levels. In this regime, the $\vec{y}$ polarized cavity field reduces to

$$\left|a_y\right|^2 = \eta^2 g^2 \mathcal{S}\frac{{p_1}^2\,\delta^2}{\kappa^2 + (\Delta_c - g^2 N_{\text{eff}}p_1\,\delta)^2}\,, \tag{S17}$$

which, for a cavity resonant with the transverse drive, yields an effective interference width $\kappa_{\text{eff}} = \kappa/(g^2 N_{\text{eff}}p_1)$. Thus, collective enhancement narrows the interference dip: for $\delta \ll \kappa_{\text{eff}}$ the photon number grows quadratically, whereas for $\delta \gg \kappa_{\text{eff}}$ it approaches a constant plateau.

### Incoherent pumping: Raman scattering

Without a systematic development of the theoretical model accounting for the Raman scattering processes, we sketch the framework of such a theory in the following. Cavity photons appear in the modes with polarizations in the $\vec{y}$ and $\vec{z}$ directions in an incoherent way, which can be treated analogously to the interaction of a boson mode with the black-body radiation [3]. The many-atom Heisenberg-Langevin equations in eq. (S9) have to be complemented by decay and

Langevin noise terms. While the prior accelerates the loss of coherence on top of the usual cavity loss channel described by $\kappa$, the latter has no mean field effect on the amplitudes $a_{y(z)}$. At the same time, there is a contribution to amplify the mean intensity $\langle a^\dagger_{y(z)} a_{y(z)} \rangle$ because the normally ordered Langevin noise terms have a non-vanishing correlation

$$\langle \xi_R^\dagger(t) \xi_R(t') \rangle = D_R \, \delta(t - t') \,, \tag{S18}$$

with a diffusion coefficient $D_R = 2\gamma_R P_e$ with $\gamma_R$ being the transition rate, and the population in the excited state is $P_e$. The proportionality of heating (i.e., diffusion) to the population in the excited state is analogous to the case of the black-body radiation where the diffusion is proportional to the mean thermal photon number $n_B$. This excited state population is suppressed by the vanishing of the collective polarizability $\mathcal{P}(\Delta^*) = 0$. The inhibition of exciting the polaritons entails thus the inhibition of Raman scattering, too.

## REFERENCES

1. P. Domokos and H. Ritsch, "Collective Cooling and Self-Organization of Atoms in a Cavity," Phys. Rev. Lett. **89**, 253003 (2002). Publisher: American Physical Society.
2. B. Gábor, A. K. Varooli, D. Varga, *et al.*, "Demonstration of strong coupling of a subradiant atom array to a cavity vacuum," EPJ Quantum Technol. **12**, 93 (2025).
3. C. Cohen-Tannoudji, J. Dupont-Roc, and G. Grynberg, *Processus d'interaction entre photons et atomes*, no. 2 in Photons et atomes (InterÉd. Ed. du CNRS, Paris, 1988).
